# Supplementary material for: Restructuring Conversations using Discourse Relations for Zero-shot Abstractive Dialogue Summarization
Source: arXiv:1902.01615 source file (2020-10-13)
Supplement: Supplementary file 1 [file ami_examples.tex]

\begin{table*}
\centering
\begin{tabular}{|p{0.9\linewidth}|}
\hline 
\textbf{BART Summary - No Discourse} \\
\hline

\hline
\textbf{BART Summary - With Discourse} \\
\hline
\hline
\end{tabular}
\caption{\label{font-table} Font guide. }
\end{table*}
